# Supplementary material for: CMSA algorithm for solving the prioritized pairwise test data generation problem in software product lines
Source: arXiv:2402.04597 source file (2024-02-07)
Supplement: Supplementary file 1 [file AppendixA.tex]

% !TEX root = ../main.tex
% Appendix A

\label{AppendixA} % For referencing this appendix elsewhere, use \ref{AppendixA}

header on each page - perhaps a shortened title
\begin{verbatim}
Best results:

Only considering prioritized products:
=====================
Apache                   :  7 (max_time=1,n_a=1,age_max=1)
BerkeleyDBFootprint      :  6 (max_time=5,n_a=1,age_max=3)
BerkeleyDBMemory         : 20 (max_time=1,n_a=1,age_max=1)
BerkeleyDBPerformance    :  9 (max_time=1,n_a=1,age_max=1)
Curl                     :  9 (max_time=1,n_a=1,age_max=1)
LinkedList               : 15 (max_time=1,n_a=1,age_max=1)
Linux                    : 10 (max_time=5,n_a=3,age_max=3)
LLVM                     :  8 (max_time=1,n_a=1,age_max=1)
PKJab                    :  6 (max_time=1,n_a=1,age_max=1)
Prevayler                :  6 (max_time=1,n_a=1,age_max=1)
SensorNetwork            : 11 (max_time=15,n_a=5,age_max=3)
SQLiteMemory             : 35 (max_time=5,n_a=1,age_max=3)
Violet                   : 17 (max_time=30,n_a=1,age_max=1)
Wget                     : 11 (max_time=5,n_a=1,age_max=1)
x264                     : 10 (max_time=5,n_a=1,age_max=5)
ZipMe                    :  6 (max_time=1,n_a=1,age_max=1)
-----------------
Mean: 11.625
Std:  7.236
-----------------



Random products:
=====================
Apache                   :  6 (max_time=3,n_a=3,age_max=4)
BerkeleyDBFootprint      :  7 (max_time=3,n_a=3,age_max=4)
BerkeleyDBMemory         : 20 (max_time=3,n_a=3,age_max=4)
BerkeleyDBPerformance    :  9 (max_time=3,n_a=3,age_max=4)
Curl                     :  8 (max_time=3,n_a=4,age_max=6)
LinkedList               : 11 (max_time=3,n_a=4,age_max=6)
Linux                    : 10 (max_time=3,n_a=3,age_max=4)
LLVM                     :  7 (max_time=3,n_a=3,age_max=5)
PKJab                    :  6 (max_time=5,n_a=3,age_max=4)
Prevayler                :  6 (max_time=3,n_a=3,age_max=4)
SensorNetwork            : 11 (max_time=3,n_a=3,age_max=6)
SQLiteMemory             : 25 (max_time=3,n_a=5,age_max=5)
Violet                   : 15 (max_time=3,n_a=4,age_max=6)
Wget                     : 10 (max_time=3,n_a=3,age_max=5)
x264                     : 10 (max_time=3,n_a=3,age_max=4)
ZipMe                    :  6 (max_time=3,n_a=3,age_max=4)
-----------------
Mean: 10.438
Std:  5.220
-----------------

Hybrid approach:
=====================
Apache                   :  6 (max_time=3,n_a=3,age_max=5)
BerkeleyDBFootprint      :  7 (max_time=3,n_a=3,age_max=4)
BerkeleyDBMemory         : 20 (max_time=3,n_a=3,age_max=4)
BerkeleyDBPerformance    :  9 (max_time=3,n_a=3,age_max=4)
Curl                     :  8 (max_time=3,n_a=5,age_max=6)
LinkedList               : 12 (max_time=3,n_a=3,age_max=6)
Linux                    :  9 (max_time=5,n_a=4,age_max=5)
LLVM                     :  7 (max_time=3,n_a=3,age_max=4)
PKJab                    :  6 (max_time=5,n_a=4,age_max=4)
Prevayler                :  6 (max_time=3,n_a=3,age_max=4)
SensorNetwork            : 11 (max_time=3,n_a=3,age_max=4)
SQLiteMemory             : 25 (max_time=3,n_a=5,age_max=5)
Violet                   : 12 (max_time=5,n_a=4,age_max=6)
Wget                     : 10 (max_time=3,n_a=3,age_max=4)
x264                     : 10 (max_time=3,n_a=3,age_max=4)
ZipMe                    :  6 (max_time=3,n_a=3,age_max=4)
-----------------
Mean: 10.250
Std:  5.130
-----------------

Best:
=====================
Apache                   :  6 (random - max_time=3,n_a=3,age_max=4)
BerkeleyDBFootprint      :  6 (prioritized - max_time=5,n_a=1,age_max=3)
BerkeleyDBMemory         : 20 (prioritized - max_time=1,n_a=1,age_max=1)
BerkeleyDBPerformance    :  9 (prioritized - max_time=1,n_a=1,age_max=1)
Curl                     :  8 (random - max_time=3,n_a=4,age_max=6)
LinkedList               : 11 (random - max_time=3,n_a=4,age_max=6)
Linux                    :  9 (hybrid - max_time=5,n_a=4,age_max=5)
LLVM                     :  7 (random - max_time=3,n_a=3,age_max=5)
PKJab                    :  6 (prioritized - max_time=1,n_a=1,age_max=1)
Prevayler                :  6 (prioritized - max_time=1,n_a=1,age_max=1)
SensorNetwork            : 11 (prioritized - max_time=15,n_a=5,age_max=3)
SQLiteMemory             : 25 (random - max_time=3,n_a=5,age_max=5)
Violet                   : 12 (hybrid - max_time=5,n_a=4,age_max=6)
Wget                     : 10 (random - max_time=3,n_a=3,age_max=5)
x264                     : 10 (prioritized - max_time=5,n_a=1,age_max=5)
ZipMe                    :  6 (prioritized - max_time=1,n_a=1,age_max=1)
-----------------
Mean: 10.125
Std:  5.158
-----------------
\end{verbatim}
