# Supplementary material for: CMSA algorithm for solving the prioritized pairwise test data generation problem in software product lines
Source: arXiv:2402.04597 source file (2024-02-07)
Supplement: Supplementary file 2 [file AppendixB.tex]

% !TEX root = ../main.tex
% Appendix B

\chapter{Source Code}

\label{AppendixB}

\lhead{Appendix B. \emph{Source Code}}

\section{CMSA}
    \subsection{cmsa.py}
    \inputminted[linenos]{python}{../prog/cmsa.py}

    \subsection{cmsa\_prioritized.py}
    \inputminted[linenos]{python}{../prog/cmsa_prioritized.py}

    \subsection{cmsa\_random.py}
    \inputminted[linenos]{python}{../prog/cmsa_random.py}

    \subsection{cmsa\_hybrid.py}
    \inputminted[linenos]{python}{../prog/cmsa_hybrid.py}

    \subsection{cmsa\_factory.py}
    \inputminted[linenos]{python}{../prog/cmsa_factory.py}
\section{Feature Model}
    \subsection{feature\_model.py}
    \inputminted[linenos]{python}{../prog/feature_model.py}

    \subsection{feature\_tree.py}
    \inputminted[linenos]{python}{../prog/feature_tree.py}
